# Supplementary material for: On Nematicity and Charge Order in Superoxygenated La$_{2-x}$Sr$_x$CuO$_{4+y}$
Source: arXiv:1707.04367 ancillary file (2017-10-03)
Supplement: Supplementary file 1 [file supplemental-material.pdf]

**Supplemental Material to**  
**“On Nematicity and Charge Order in Superoxygenated  $\text{La}_{2-x}\text{Sr}_x\text{CuO}_{4+y}$ ”**

Zhiwei Zhang,<sup>1</sup> R. Sutarto,<sup>2</sup> F. He,<sup>2</sup> F. C. Chou,<sup>3</sup> L. Udby,<sup>4</sup> S. L.  
Holm,<sup>4</sup> Z. H. Zhu,<sup>5</sup> W. A. Hines,<sup>1</sup> J. I. Budnick,<sup>1</sup> and B. O. Wells<sup>1</sup>

<sup>1</sup>*Department of Physics, University of Connecticut, Storrs CT 06269, USA*

<sup>2</sup>*Canadian Light Source, Saskatoon, Saskatchewan S7N 2V3, Canada*

<sup>3</sup>*Center for Condensed Matter Sciences, National Taiwan University, Taipei 10670, Taiwan*

<sup>4</sup>*X-ray and Neutron Science, Niels Bohr Institute,  
University of Copenhagen, DK-2100 Copenhagen, Denmark*

<sup>5</sup>*Department of Physics, Massachusetts Institute of Technology, Cambridge MA 02139, USA*

In this Supplemental Material, various supportive details regarding the facts, figures and arguments in the main article are provided and presented in the following sections.

### O XAS FITTING PROFILE FOR THE SAMPLES

Fig. S1A plots the O XAS spectra for the two samples used in this work, labelled LCO+O, LSCO+O, along with two XAS plots for LSCO doped to 0.10 and 0.15 holes per Cu from Ref. [1]. In Ref. [1] those are adjacent doping levels plotted, and the two of most interest here. As discussed in the main article, the ratio between the intensities of MCP, near 528.5 eV, and the UHB peak, near 531 eV, depends on the hole doping level. Detailed differences in the lineshapes can lead to small differences in the extracted lineshapes of the unresolved peaks, making a rigorously quantitative comparison between our work and the reference impossible. However, a qualitative comparison indicates that our more highly doped sample, labelled LSCO+O, has a similar but slightly higher doping level than the  $x=0.15$  sample from the reference. The lesser doped sample studied here, labelled LCO+O, is clearly more highly doped than the  $x=0.10$  sample but less than the  $x=0.15$  sample from the reference. Fig. S1B gives the normalized XAS measured in TEY at the O  $K$  pre-edges for both charge-ordered LCO+O and non-charge-ordered LSCO+O samples. The normalized data were obtained by first subtracting the components of the absorption from the hybridization states near 532 eV and the main  $K$  edge at higher energies, and then normalizing both to equal energy-integrated intensity. The higher doping level in LSCO+O is quite clear. Based upon the data in Ref. [1] we estimate the difference in doping of the two samples to be near 0.03 holes per Cu and thus the LCO+O sample near 0.125 holes and the LSCO+O sample near 0.16 (rounded).

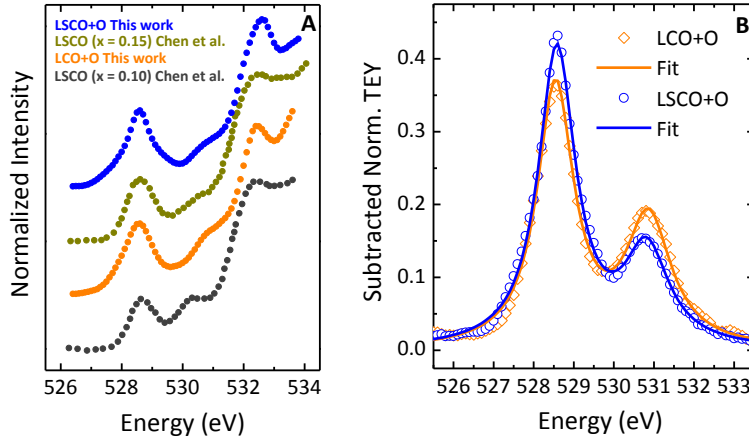

FIG. S1. **A.** Raw data of XAS at O edges for LCO+O, LSCO+O and LSCO with 0.10 and 0.15 doping levels from Ref. [1]. Here all the spectra were normalized to a universal main  $K$  edge height. **B.** The normalized TEY at MCP and UHB for both LCO+O and LSCO+O samples, plotted in orange and blue respectively.

### H SCANS UNDER DIFFERENT TEMPERATURES

Fig. S2 shows a set of  $H$  scans of  $(H\ 0\ 1.55)$  under different temperatures from 20K to 300K. These are the raw scans that led to the temperature dependent data plotted in Fig. 2A of the main article. The peaks are fit to Lorentzian shapes. A well-defined CO peak appears at  $H = 0.247$  when the temperature is below  $T = 50$ K. We estimate a transition temperature near  $\sim 50$ K based upon the temperature dependence of the peak intensities at lower temperatures.

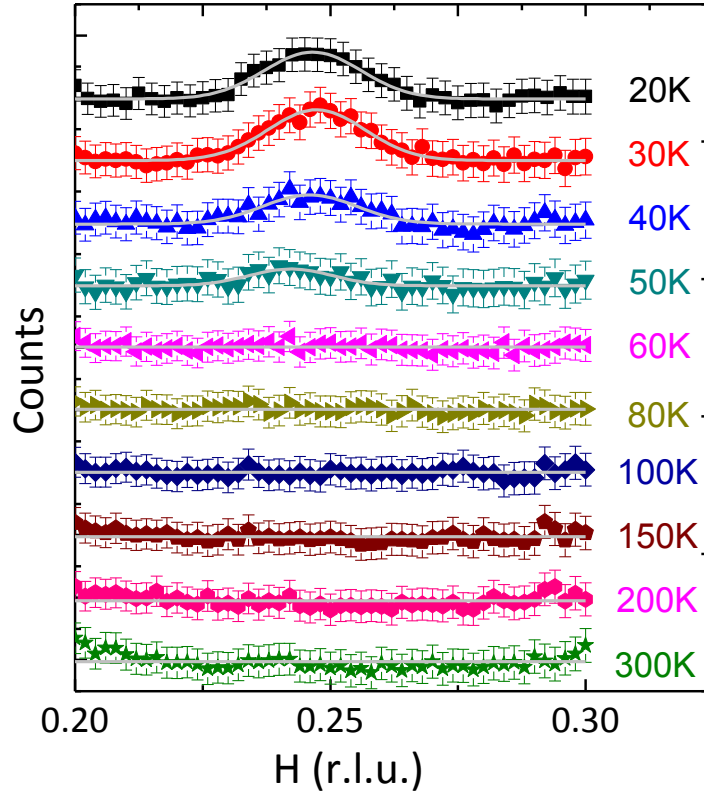

FIG. S2.  $H$  scans of the resonant CO peaks ( $H\ 0\ 1.55$ ) at Cu  $L_3$  edge under various temperatures from 20K to 300K. The presented data were background subtracted. All data were fit to Lorentzian peak shapes.

### FORM FACTORS OF CO SCATTERING EXTRACTED BY XAS

The energy dependence of the scattering form factors were extracted from the TEY XAS at  $Q_{CO}$ . Fig. S3A shows the TEY XAS at 60K. The Cu  $L_3$  edge peak appears at  $E = 931.5$  eV.

The total scattering form factor can be written as,

$$f(E) = f'(E) + if''(E) \quad (1)$$

where  $f'(E)$  and  $f''(E)$  are the real and imaginary part of the total form factor, respectively. Using the Chantler table[2], one is able to tabulate  $f''(E)$ , which is shown in Fig. S3B. It is found that at Cu  $L_3$  edge,  $f'' \sim 145$  electrons/atom. Further by Kramers-Kronig transformation,  $f'(E)$  is found and the energy dependence was plotted in Fig. S3C.

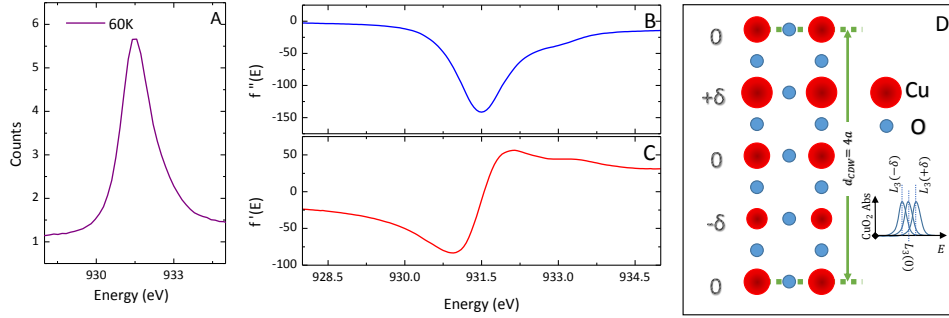

FIG. S3. Calculated absorption scattering form factors at the Cu  $L_3$  edge range at 60K for the charge-ordered sample. **A.** The XAS measured in TEY at the Cu  $L_3$  edge. **B(C).** Energy dependence of the imaginary(real) part of the total form factor across the Cu  $L_3$  edge. **D.** Schematics for energy-shift model in allowing charge order scattering.

With these energy-dependent form factors at hand, one is able to calculate the energy dependence of the CO scattering using the energy-shift model.[3] As described by the model, sites with different doped charge densities have different Cu  $L_3$  absorption energies. As shown in Fig. S3D, form factors of Cu associated with different absorption energies are then shifted according to the actual absorption energies. The form factors for Cu with different dopants are

$$f_0(E) = f(E) \quad (2)$$

$$f_{+\delta}(E) = f_0(E + \Delta E) \quad (3)$$

$$f_{-\delta}(E) = f_0(E - \Delta E) \quad (4)$$

The form factors of O and La can be treated constant as Cu  $L_3$  edge is far from the absorption energies of both elements. Since the scattering intensity  $I(E) \propto \frac{|S(E)|^2}{\mu}$ ,

$$I(E) \propto \frac{1}{\mu} |f(E + \Delta E) - f(E - \Delta E)|^2 \quad (5)$$

In this work's calculation, the shift in energy is  $\Delta E = 0.05$  eV.

### ENERGY DEPENDENCE OF THE CHARGE ORDER

In order to extract the energy dependence of the CO scattering intensity we used the difference between a fixed  $Q$  scan at 20 K versus another at 60 K where the CO peak is gone. Fig. S4A shows the scans in energy with  $Q$  fixed on the peak at the  $Q_{CO} = (0.247, 0, 1.55)$ , measured in total fluorescence yield (TFY). At 60K the intensity is purely the non-ordering fluorescence response whereas at 20K the intensity is a sum of the non-ordering fluorescence response and the CO scattering response. Fig. S4B plots the TFY at 931.5 eV (the height of the peaks in Fig. S4A) as a function of the temperature. The red dotted curve is a guide to the eye and makes clear the extra intensity associated with CO below  $\sim 50$ K.

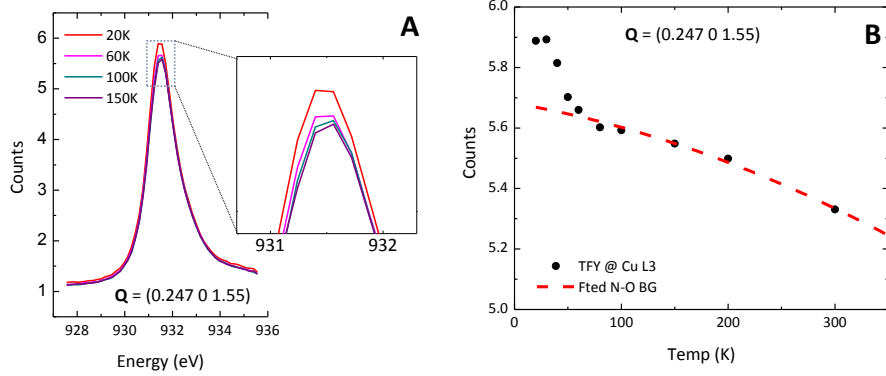

FIG. S4. **A.** Total fluorescence yields at CO under different temperatures. A significant height increase at the Cu  $L_3$  edge at 20K compared to 60K and above is due to the contribution by the CO scattering. **B.** Total fluorescence yield at CO at Cu  $L_3$  edge as a function of temperature. The non-ordering resonant fluorescence background is fitted to a polynomial function. The units are arbitrary but are comparable between these two figures.

The energy dependence of the CO intensity is plotted in Fig. 2B of the main article. Our energy-shift model calculation shows an excellent fit to the experimental data.

# WEAK EVIDENCE OF CHARGE ORDER RESONANCE AT O MCP

Our manuscript only described CO as measured at the Cu  $L_3$  edge. We also searched for CO at the O K edge prepeak known as the MCP. The data was inconclusive, as shown in Fig. S5. We are not able to clearly state whether this represents a proper CO peak.

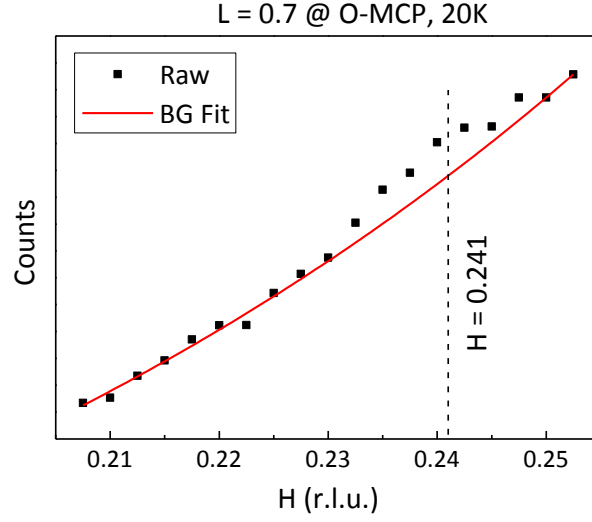

FIG. S5. Possible resonant CO peak at MCP absorption edge.

**(001) REFLECTION: ABSENCE IN CHARGE-ORDERED LCO+O AND THE  
EXTRACTION METHODOLOGY IN LSCO+O**

In this section we provide the evidence for the lack of an (001) resonant peak in the LCO+O sample and how we extracted the resonant portion of the (001) peak in the more heavily doped LSCO+O sample. Fig. S6 shows the raw data for  $L$ -scans at 523.5 eV (below MCP by 5 eV), 528.5 eV (MCP) and 532.5 eV (main  $K$  edge). The inset indicates these chosen energies in the absorption spectrum. The peak at 523.5 eV is the (002) peak from unavoidable higher order light, as this energy is before the absorption edge and the (001) peak is not allowed off resonance. The (002) peak itself will not resonate in this range, as there are no absorption edges at twice the O  $K$  edge near 1050 eV. Thus, the contribution from higher order light should be constant over this small energy range. If a resonant (001) reflection exists, extra intensity should appear above that for the (002) with higher order light. Further, the width for a resonant (001) peak, particularly for an effect such as nematic order, would be significantly larger than for the (002) Bragg peak. However, we did not observe any intensity increase or width increase at MCP as in Ref. [4] due to nematic order or at main  $K$  edge as reported in Ref. [5] due to LTT octahedral tilting. Table S1 gives detailed fitting profiles for the scans. Further, we detected no Cu  $L$  or La  $M$  resonant (001) peak either. We conclude that there is no nematic order as defined in Ref. [4], and that the LCO+O sample is indeed in the LTO phase.

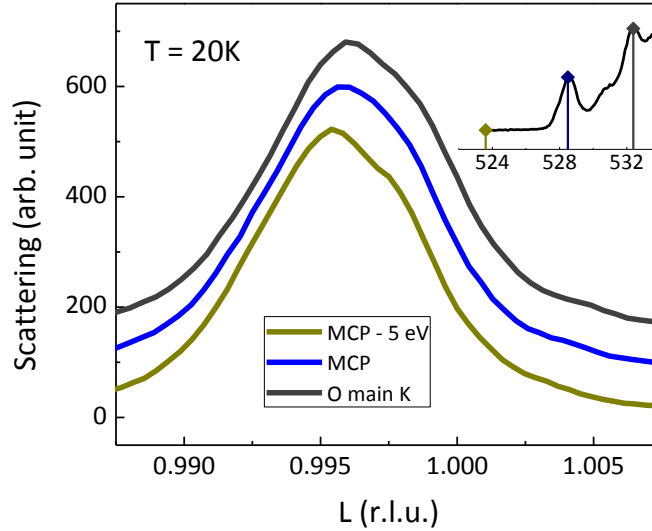

FIG. S6. LCO+O:  $L$ -scans at different energies. The inset shows the chosen energies in the absorption spectrum.

TABLE S1. Fitting profiles for  $L$ -scans at different energies for LCO+O.

| Energy (eV)           | 523.5  | 528.5  | 532.5  | 965    |
|-----------------------|--------|--------|--------|--------|
| $Q$                   | (001)  | (001)  | (001)  | (002)  |
| FWHM (r.l.u. in $L$ ) | 0.0074 | 0.0074 | 0.0077 | 0.0070 |
| Intensity             | 682    | 705    | 749    | 3022   |

In LSCO+O, we observed a (001) reflection at the O  $K$  edge that is robust up to at least 70K, well above the transition temperature for charge order. Table S2 shows the fitting profile for the  $L$ -scans at several selective energies across the O  $K$  edge. A significant width increase and intensity increase happens at 532.0 eV.

TABLE S2. Fitting profiles for  $L$ -scans at different energies for LSCO+O.

| Energy (eV)           | 528.1  | 528.5  | 532.0  | 532.5  | 535.2  |
|-----------------------|--------|--------|--------|--------|--------|
| $Q$                   | (001)  | (001)  | (001)  | (001)  | (001)  |
| FWHM (r.l.u. in $L$ ) | 0.0053 | 0.0052 | 0.0087 | 0.0078 | 0.0057 |
| Intensity             | 896    | 868    | 2753   | 2046   | 1183   |

Again, there is a contribution from the (002) reflection with higher order light, but we can subtract out the resonant contribution. Since at 528.1 eV, the peak is only from the higher order light, it is valid to extract the (001) reflection at the maximum resonance (532.0 eV) by subtracting the  $L$ -scan at 528.1 eV from the one at 532.0 eV.

TABLE S3. Table for the transition temperature, correlations length (in  $1/\text{HWHM}$ ) for charge order and spin order in various 214 cuprates.

| Material     | $T_{\text{SO}}/\text{K}$ | $\xi/\text{\AA}$ | Technique      | Reference                    | $T_{\text{CO}}/\text{K}$ | $\xi/\text{\AA}$ | Technique  | Reference                  |
|--------------|--------------------------|------------------|----------------|------------------------------|--------------------------|------------------|------------|----------------------------|
| LCO+O        | 40                       | 300              | Neutron        | Udby <i>et al.</i> [6]       | 50                       | 60               | RXS        | This Work                  |
| LSCO         | 40                       | 400              | Neutron        | Yamada <i>et al.</i> [7]     | 75                       | 30               | Hard X-ray | Croft <i>et al.</i> [8]    |
| Surface LSCO |                          |                  |                |                              | 55                       | 40               | RXS        | Wu <i>et al.</i> [9]       |
| LBCO         | 40                       | 480              | Neutron        | Huecker <i>et al.</i> [10]   | 52                       | 255              | Hard X-ray | Wilkins <i>et al.</i> [11] |
|              |                          |                  |                |                              | 48                       | 300              | RXS        | Achkar <i>et al.</i> [4]   |
| LNSCO        | 38                       | 120              | Neutron        | Tranquada <i>et al.</i> [12] | 52                       | 111              | Hard X-ray | Wilkins <i>et al.</i> [11] |
| LESCO        | 30                       |                  | $\mu\text{SR}$ | Klauss <i>et al.</i> [13]    | 80                       | 320              | RXS        | Fink <i>et al.</i> [14]    |

### A COMPLETE LITERATURE REVIEW OF FACTS FOR STRIPES IN 214 CUPRATES

Stripe like charge and spin order has been reported for most 214-type cuprate samples doped near  $1/8$ th hole per Cu. Here we prepared Table S3 for a comparison between different 214 samples.

- 
- [1] C. T. Chen, F. Sette, Y. Ma, M. Hybertsen, E. Stechel, W. Foulkes, M. Schulter, S. Cheong, A. Cooper, L. Rupp, B. Batlogg, Y. Soo, Z. Ming, A. Krol, and Y. Kao, *Phys. Rev. Lett.* **66**, 104 (1991).
  - [2] C. T. Chantler, *J. Phys. Chem. Ref. Data* **24**, 71 (1995).
  - [3] A. J. Achkar, F. He, R. Sutarto, J. Geck, H. Zhang, Y.-J. Kim, and D. G. Hawthorn, *Phys. Rev. Lett.* **110**, 017001 (2013).
  - [4] A. J. Achkar, M. Zwiebler, C. McMahon, F. He, R. Sutarto, I. Djianto, Z. Hao, M. J. P. Gingras, M. Hücker, G. D. Gu, A. Revcolevschi, H. Zhang, Y.-J. Kim, J. Geck, and D. G. Hawthorn, *Science* **351**, 576 (2016).
  - [5] J. Fink, V. Soltwisch, J. Geck, E. Schierle, E. Weschke, and B. Büchner, *Phys. Rev. B* **83**, 092503 (2011).
  - [6] L. Udby, J. Larsen, N. B. Christensen, M. Boehm, C. Niedermayer, H. E. Mohottala, T. B. S. Jensen, R. Toft-Petersen, F. C. Chou, N. H. Andersen, K. Lefmann, and B. O. Wells, *Phys. Rev. Lett.* **111**, 227001 (2013).
  - [7] K. Yamada, C. H. Lee, K. Kurahashi, J. Wada, S. Wakimoto, S. Ueki, H. Kimura, Y. Endoh, S. Hosoya, G. Shirane, R. J. Birgeneau, M. Greven, M. A. Kastner, and Y. J. Kim, *Phys. Rev. B* **57**, 6165 (1998).
  - [8] T. P. Croft, C. Lester, M. S. Senn, A. Bombardi, and S. M. Hayden, *Phys. Rev. B* **89**, 224513 (2014).
  - [9] H.-H. Wu, M. Buchholz, C. Trabant, C. F. Chang, A. C. Komarek, F. Heigl, M. v. Zimmermann, M. Cwik, F. Nakamura, M. Braden, and C. Schüßler-Langeheine, *Nat. Commun.* **3**, 1023 (2012).
  - [10] M. Hücker, M. v. Zimmermann, G. D. Gu, Z. J. Xu, J. S. Wen, G. Xu, H. J. Kang, A. Zheludev, and J. M. Tranquada, *Phys. Rev. B* **83**, 104506 (2011).
  - [11] S. B. Wilkins, M. P. M. Dean, J. Fink, M. Hücker, J. Geck, V. Soltwisch, E. Schierle, E. Weschke, G. Gu, S. Uchida, N. Ichikawa, J. M. Tranquada, and J. P. Hill, *Phys. Rev. B* **84**, 195101 (2011).
  - [12] J. M. Tranquada, G. D. Gu, M. Hücker, Q. Jie, H.-J. Kang, R. Klingeler, Q. Li, N. Tristan, J. S. Wen, G. Y. Xu, Z. J. Xu, J. Zhou, and M. v. Zimmermann, *Phys. Rev. B* **78**, 174529 (2008).
  - [13] H.-H. Klauss, W. Wagener, M. Hillberg, W. Kopmann, H. Walf, F. J. Litterst, M. Hücker, and B. Büchner, *Phys. Rev. Lett.* **85**, 4590 (2000).
  - [14] J. Fink, E. Schierle, E. Weschke, J. Geck, D. Hawthorn, V. Soltwisch, H. Wadati, H.-H. Wu, H. A. Dürr, N. Wizen, B. Büchner, and G. A. Sawatzky, *Phys. Rev. B* **79**, 100502 (2009).
